# Supplementary material for: Laser induced persistent orientation of chiral molecules
Source: arXiv:1905.12609 ancillary file (2019-07-23)
Supplement: Supplementary file 1 [file sup_mat.pdf]

# Supplementary Material for "Laser induced persistent orientation of chiral molecules"


Ilia Tutunnikov,[1,*] Johannes Floß,[2,*] Erez Gershnabel,[1] Paul Brumer,[2,†] and Ilya Sh. Averbukh[1,‡]

[1] *AMOS and Department of Chemical and Biological Physics, Weizmann Institute of Science, Rehovot 7610001, Israel*

[2] *Chemical Physics Theory Group, Department of Chemistry, and Center for Quantum Information and Quantum Control, University of Toronto, Toronto, Ontario M5S 3H6, Canada*


## Molecular Parameters

Supplementary Table I summarizes the molecular parameters of ($R$)-PPO used in our simulations.

| Molecule | Moments of inertia | Polarizability tensor components | Dipole moment components |
|---|---|---|---|
| | $I_a = 180386$ | $\alpha_{aa} = 45.63$ $\alpha_{ab} = 2.56$ | $\mu_a = 0.965$ |
| ($R$)-PPO | $I_b = 493185$ | $\alpha_{bb} = 37.96$ $\alpha_{ac} = 0.85$ | $\mu_b = -1.733$ |
| | $I_c = 553513$ | $\alpha_{cc} = 37.87$ $\alpha_{bc} = 0.65$ | $\mu_c = 0.489$ |

**Supplementary Table I**. Summary of molecular properties: eigenvalues of the moment of inertia tensor (atomic units), components of polarizability tensor (atomic units) and components of dipole moment (Debye) in the body-fixed frame of molecular principal axes. For the complimentary enantiomers, the values of $\alpha_{ac}$, $\alpha_{bc}$ and $\mu_c$ have the opposite sign. The molecular electronic properties were computed using GAUSSIAN software package (method: CAM-B3LYP/aug-cc-pVTZ) [1].

## Derivation of Equation 1

As discussed in the main text, we consider an excitation by a pair of delayed cross-polarized laser pulses. The first pulse is polarized along the laboratory $X$ axis, while the polarization of the second one is in the $XY$ plane at $+\pi/4$ to the $X$ axis. We assume that the first pulse induces a perfect alignment of the most polarizable molecular axis ($x_1$) along $X$ axis. Initially, we consider only half of all molecules, in which the most polarizable axis points along $+X$ [see Fig. 1(a)]. Angle $\varphi \in [0, 2\pi)$ is the angle between the $Y$ axis and the $x_2$ axis. lying in the $YZ$ plane [see Sup. Fig. 1(b)]. The aligned molecules are uniformly distributed in $\varphi$. The interaction potential, $U$ and torque, $\mathbf{T}$ induced by a non-resonant optical field are given by

$$U = -\frac{1}{2} \langle \mathbf{d}_{\text{ind}} \cdot \mathbf{E} \rangle \qquad \mathbf{T} = \langle \mathbf{d}_{\text{ind}} \times \mathbf{E} \rangle , \tag{1}$$

where the angle brackets denote time averaging over the optical cycle, $\mathbf{d}_{\text{ind}} = \boldsymbol{\alpha}\mathbf{E}$ is the induced dipole, $\boldsymbol{\alpha}$ is the polarizability tensor, and $\mathbf{E}$ is the vector of the electric field. The duration of the laser pulses is assumed to be short as compared to the typical rotation periods of the chiral molecules, therefore the effect of the second pulse is considered in the impulsive approximation, $\Delta\mathbf{L} \propto \mathbf{T}$.


* I. T. and J. F. contributed equally to this work.
† paul.brumer@utoronto.ca
‡ ilya.averbukh@weizmann.ac.il


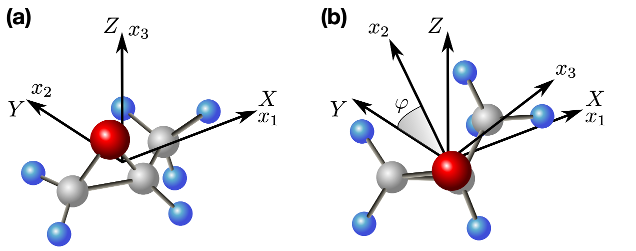


**Supplementary Figure 1**. **(a)** The frame of polarizability principal axes $x_1$, $x_2$ and $x_3$ ($\alpha_{33} < \alpha_{22} < \alpha_{11}$) coincides with the laboratory fixed frame. **(b)** The molecule is rotated (about $X$) by an angle $\varphi$, measured from the positive $Y$ axis to positive $x_2$ axis, lying in the $YZ$ plane.

The second pulse (twisted with respect to the first one) induces unidirectional rotation in the $XY$ plane resulting in orientation of $\langle \boldsymbol{\ell} \rangle$ along $Z$, which constitutes the first criterion for the long-lasting orientation. In addition, there is an orienting torque acting on the aligned most polarizable axis, $x_1$. To check whether the second criterion for the long-lasting orientation is satisfied, we evaluate the torques along the molecular $a$ and $c$ axes. For this, we begin from transforming the electric field coordinates from the laboratory frame of reference to the frame of polarizability tensor principal axes

$$\mathbf{E}_{\boldsymbol{\alpha}} \propto R_X(-\varphi) \begin{pmatrix} 1 \\ 1 \\ 0 \end{pmatrix}, \tag{2}$$

where $\mathbf{E}_{\boldsymbol{\alpha}}$ denotes the column vector of electric field coordinates in the frame of polarizability tensor principal axes, $(1,1,0)^T$ represents the second pulse lying in the $XY$ plane at $+\pi/4$ angle, and $R_X(\theta)$ is the canonical rotation matrix. We evaluate the torque, using

$$\mathbf{T}_{\boldsymbol{\alpha}} \propto \left[ \begin{pmatrix} \alpha_{11} & 0 & 0 \\ 0 & \alpha_{22} & 0 \\ 0 & 0 & \alpha_{33} \end{pmatrix} \mathbf{E}_{\boldsymbol{\alpha}} \right] \times \mathbf{E}_{\boldsymbol{\alpha}} \tag{3}$$

The torque is transformed to the frame of inertia tensor principal axes by an orthogonal matrix $R$, defined by $\mathbf{v}_{\mathbf{I}} = R\mathbf{v}_{\boldsymbol{\alpha}}$, where $\mathbf{v}_{\mathbf{I}}$ denotes the column vector of coordinates of some vector $\vec{v}$ in the frame of inertia tensor principal axes. In the frame of principal axes of inertia tensor the torque is given by

$$\mathbf{T}_{\mathbf{I}} \equiv \begin{pmatrix} \tau_a \\ \tau_b \\ \tau_c \end{pmatrix} \propto R\mathbf{T}_{\boldsymbol{\alpha}}. \tag{4}$$

For the transformation, we order the inertia principal axes as $abc$, while the order of polarizability principal

axes is chosen to be $x_1x_3x_2$. Since the molecule is chiral, polarizability tensor principal axes and inertia tensor principal axes frames do not align [see Fig. 1(a) in the main text] and $R$ is not diagonal

$$R = \begin{pmatrix} R_{a1} & R_{a3} & R_{a2} \\ R_{b1} & R_{b3} & R_{b2} \\ R_{c1} & R_{c3} & R_{c2} \end{pmatrix} \tag{5}$$

The explicit expression for $\tau_k$ ($k = a, c$) is given by Eq. 1 (in the main text) $\tau_k \propto C_k \sin(2\varphi) + D_k \sin(\varphi + \phi_k)$, where $C_k = (\alpha_{33} - \alpha_{22}) R_{k1}/2$, $D_k = \sqrt{A_k^2 + B_k^2}$, $A_k = (\alpha_{11} - \alpha_{33}) R_{k2}$, $B_k = (\alpha_{11} - \alpha_{22}) R_{k3}$, and $\cos(\phi_k) = A_k/D_k$. When the off-diagonal elements of $R$ differ from zero, the subdomains of positive and negative $\tau_k$ in the interval $\varphi \in [0, 2\pi)$ are not equal, which is precisely the required $T_k^+$ vs $T_k^-$ asymmetry. When the two frames do coincide (non-chiral molecule), $R$ becomes diagonal resulting in torques $\tau_a = C_a \sin(2\varphi)$ and $\tau_c = A_c \sin(\varphi)$. In this case, the $T_k^+$ vs $T_k^-$ symmetry is preserved.

## Quantum Mechanical Simulation

For our quantum mechanical simulations of the laser driven dynamics of the chiral molecules, we used the following expressions for the envelopes of the short pulses

$$\varepsilon^2(t)/\mathcal{E}_0^2 = \begin{cases} \cos^2\left(\frac{\pi}{2}\frac{t-t_0}{\mathrm{FWHM}}\right) & |t - t_0| \leq \mathrm{FWHM} \\ 0 & \text{otherwise,} \end{cases} \tag{6}$$

and the optical centrifuge

$$\varepsilon^2(t)/\mathcal{E}_0^2 = \begin{cases} \sin^2\left(\frac{\pi t}{2t_{\mathrm{on}}}\right) & 0 \leq t < t_{\mathrm{on}} \\ 1 & t_{\mathrm{on}} \leq t < t_{\mathrm{p}} - t_{\mathrm{off}} \\ \sin^2\left[\frac{\pi(t-t_{\mathrm{p}})}{2t_{\mathrm{off}}}\right] & t_{\mathrm{p}} - t_{\mathrm{off}} \leq t < t_{\mathrm{p}} \\ 0 & t_{\mathrm{p}} \leq t \end{cases}. \tag{7}$$

The first step in our numerical scheme is to express the Hamiltonian in the basis of symmetric-top wave functions $|JKM\rangle$. Here, the quantum number $J$ is the total angular momentum, $K$ is its projection onto the molecule-fixed $c$-axis, and $M$ is its projection onto the space-fixed $Z$-axis. The non-zero matrix elements of asymmetric-top rotational Hamiltonian are given by [4]

$$\langle JKM|H_{\mathrm{rot}}|JKM\rangle = \frac{C+A}{2}\left[J(J+1) - K^2\right] + BK^2$$
$$\langle JKM|H_{\mathrm{rot}}|JK \pm 2M\rangle = \frac{C-A}{4} \cdot f(J, K \pm 1), \tag{8}$$

where

$$f(J, K) = \sqrt{(J^2 - K^2)[(J+1)^2 - K^2]}, \tag{9}$$

and $A = \hbar^2/(2I_a)$, $B = \hbar^2/(2I_b)$, and $C = \hbar^2/(2I_c)$ are the rotational constants. Note that $H_{\mathrm{rot}}$ couples only levels with different $K$'s, therefore the asymmetric top eigenfunctions can be expressed as $|J\tau M\rangle = \sum_K c_K^{(J,\tau,M)} |JKM\rangle$, where $\tau$ enumerates the "asymmetric top" levels [4]. The coefficients $c_K^{(J,\tau,M)}$ are determined by numerically diagonalizing $H_{\mathrm{rot}}$. Note that the eigenenergies $E_{J,\tau}$ are degenerate in the quantum number $M$. The interaction potentials with the laser fields is given by $V = -\langle \mathbf{E} \cdot \mathbf{d}_{\mathrm{ind}} \rangle/2 = -\langle \mathbf{E} \cdot (\boldsymbol{\alpha}\mathbf{E}) \rangle/2$, where the angle brackets denote time averaging over the optical cycle, $\mathbf{d}_{\mathrm{ind}} = \boldsymbol{\alpha}\mathbf{E}$ is the induced dipole, $\boldsymbol{\alpha}$ is the polarizability tensor, and $\mathbf{E}$ is the vector of the electric field. It is beneficial to work in spherical basis [2, 4], in which case the transformation law for vectors/tensor has a simple form

$$T_p^{(r)} = \sum_q D_{p,q}^{(r)*} T_q^{(r)}, \tag{10}$$

where $T_p^{(r)}$ is a spherical tensor of rank $r$, indices $p$ and $q$ are associated with the laboratory and molecules fixed frames, respectively. $D_{p,q}^{(r)*}(\Omega)$ is the conjugate of the Wigner D-matrix, $\Omega$ denotes the set of three Euler angles. Note that for convenience, we suppress the angle dependence of the Wigner D-matrices. In spherical basis, the double contraction required in evaluation of the potential is given by [2]

$$V = -\frac{1}{2}\sum_{r=0}^{2}\sum_{k=-r}^{r} (-1)^k \langle A_{\mathrm{lab},k}^{(r)} \rangle \alpha_{\mathrm{lab},-k}^{(r)}, \tag{11}$$

We chose to evaluate the potential in the laboratory fixed frame. Here the angle brackets denote averaging over the optical cycle, $\alpha_{\mathrm{lab},-k}^{(r)}$ are the spherical tensor elements of molecular polarizabilty in the laboratory frame, $A_{\mathrm{lab},k}^{(r)}$ is the same for the electric field vector. Using the spherical basis, we evaluate the potential in the laboratory fixed frame. $A_{\mathrm{lab},k}^{(r)}$'s are given by

$$\begin{aligned} A_{\mathrm{lab},0}^{(0)} &= -\frac{1}{\sqrt{3}}\mathbf{E} \cdot \mathbf{E} \\ A_{\mathrm{lab},0}^{(2)} &= \frac{1}{\sqrt{6}}\left(3E_Z^2 - \mathbf{E} \cdot \mathbf{E}\right) \\ A_{\mathrm{lab},\pm1}^{(2)} &= \mp\left(E_X E_Z \pm iE_Y E_Z\right) \\ A_{\mathrm{lab},\pm2}^{(2)} &= \frac{1}{2}\left(E_X^2 - E_Y^2 \pm i2E_X E_Y\right). \end{aligned} \tag{12}$$

while the polarizability requires transformation from the molecular to the laboratory frame, $\alpha_{\mathrm{lab},p}^{(r)} = \sum_q D_{p,q}^{(r)*} \alpha_{\mathrm{mol},q}^{(r)}$ and

$$\begin{aligned} \alpha_{\mathrm{mol},0}^{(0)} &= -\frac{1}{\sqrt{3}}\left(\alpha_{aa} + \alpha_{bb} + \alpha_{cc}\right) \\ \alpha_{\mathrm{mol},0}^{(2)} &= \frac{1}{\sqrt{6}}\left(2\alpha_{cc} - \alpha_{aa} - \alpha_{bb}\right) \\ \alpha_{\mathrm{mol},\pm1}^{(2)} &= \mp\alpha_{ac} - i\alpha_{bc} \\ \alpha_{\mathrm{mol},\pm2}^{(2)} &= \frac{1}{2}\left(\alpha_{aa} - \alpha_{bb} \pm 2i\alpha_{ab}\right) \end{aligned}. \tag{13}$$

$\alpha_{ij}$'s are the Cartesian component of the polarizability tensor in the frame of inertia tensor principal axes (see Table I in the main text). The potential is given by [3]

$$V = -\frac{|\varepsilon(t)|^2}{4}\left[-\frac{1}{\sqrt{3}}\alpha_{\mathrm{mol},0}^{(0)} D_{0,0}^{(0)*} - \frac{1}{\sqrt{6}} D_{0,k}^{(2)*} \alpha_{\mathrm{mol},k}^{(2)} + \frac{\alpha_{\mathrm{mol},k}^{(2)}}{2}\left(e^{i2\gamma} D_{-2,k}^{(2)*} + e^{-i2\gamma} D_{2,k}^{(2)*}\right)\right], \tag{14}$$

where summation over the repeated index $k = -2, \ldots, 2$ is implied. The time averaging over the optical

cycle adds an overall factor of 1/2 (included). The field envelope $\varepsilon(t)$ appearing in the above is defined by Sup. Eqs. 6 and 7. The expression is valid for laser fields polarized in the $XY$-plane with $\gamma$ being the angle between the instantaneous polarization axis and the $X$-axis. In the double pulse scheme, the angle $\gamma = \pi/4$, while in case of the optical centrifuge the angle is time-dependent $\gamma = \beta t^2$. To calculate the couplings $\langle JKM|V|J'K'M'\rangle$, we use the relation [4]

$$\langle JKM|D^{(s)*}_{p,q}|J'K'M'\rangle = (-1)^{M-K}\sqrt{(2J+1)(2J'+1)} \times \begin{pmatrix} J & s & J' \\ -M & p & M' \end{pmatrix} \begin{pmatrix} J & s & J' \\ -K & q & K' \end{pmatrix}, \tag{15}$$

where the large brackets denote Wigner 3-j symbols.

To calculate the dynamics during the laser pulse, we solve the time-dependent Schrödinger equation. In particular, the rotational wave function is expressed as a linear combination of the symmetric top wave functions, $|\Psi(t)\rangle = \sum_{JKM} c_{JKM}(t)\,|JKM\rangle$, and the resulting set of coupled differential equations for the coefficients $c_{JKM}(t)$ is solved by numerical integration. To calculate the dynamics in the absence of a laser pulse, we express the wave function in the eigenbasis of $H_{\rm rot}$ (see Sup. Eq. 8), in which the field-free time-evolution is simply given as

$$\Psi(t+\Delta t) = \sum_{J,\tau,M} c_{J\tau M} e^{-iE_{J,\tau}t/\hbar}\,|J,\tau,M\rangle\,, \tag{16}$$

with

$$c_{J\tau M} = \sum_K c_K^{(J,\tau,M)*} c_{JKM}. \tag{17}$$

The polarization is given as the expectation value

$$P\left(t\right) \equiv \langle \boldsymbol{\mu}\cdot\hat{\mathbf{Z}}\rangle\left(t\right) = \langle\Psi(t)|D^{(1)*}_{0,q}\,\mu^{(1)}_{{\rm mol},q}|\Psi(t)\rangle\,, \tag{18}$$

where summation over the repeated index $q = -1, 0, 1$ is implied. The spherical tensor components of the molecular dipole are given in terms of components of the dipole expressed in the Cartesian frame of inertia tensor principal axes $\mu^{(1)}_{{\rm mol},\pm1} = \left(\mp\mu_a - i\mu_b\right)/\sqrt{2}$ and $\mu^{(1)}_{{\rm mol},0} = \mu_c$.

The alignment of the most polarizable axis, $\mathbf{m}$ towards the $X$-axis is given by the expectation value $O\left(t\right) \equiv \langle(\mathbf{m}(t)\cdot\hat{\mathbf{X}})^2\rangle$. To use the spherical basis formulas introduced above, we rewrite the alignment factor in a double contraction format (like the potential) $(\mathbf{m}\cdot\hat{\mathbf{X}})^2 = \mathbf{m}\cdot(\boldsymbol{\chi}\mathbf{m})$, where $\boldsymbol{\chi}$ is an operator that extracts the $X$ component of the vector $\mathbf{m}$. Now, we can use $(\mathbf{m}\cdot\hat{\mathbf{X}})^2 = \sum_{r=0}^{2}\sum_{k=-r}^{r}\left(-1\right)^k A^{(r)}_{{\rm mol},k}\chi^{(r)}_{{\rm mol},-k}$. The Cartesian representation of $\boldsymbol{\chi}$ in the laboratory fixed frame is given by the matrix

$$\chi_{\rm lab} = \begin{pmatrix} 1 & 0 & 0 \\ 0 & 0 & 0 \\ 0 & 0 & 0 \end{pmatrix}, \tag{19}$$

therefore its components in the spherical basis are

$$\begin{aligned} \chi^{(0)}_{{\rm lab},0} &= -\frac{1}{\sqrt{3}}\left(\chi_{XX}+\chi_{YY}+\chi_{ZZ}\right) = -\frac{1}{\sqrt{3}} \\ \chi^{(2)}_{{\rm lab},0} &= \frac{1}{\sqrt{6}}\left(2\chi_{ZZ}-\chi_{XX}-\chi_{YY}\right) = -\frac{1}{\sqrt{6}} \\ \chi^{(2)}_{{\rm lab},\pm1} &= \mp\left(\chi_{XZ}\pm i\chi_{YZ}\right) = 0 \\ \chi^{(2)}_{{\rm lab},\pm2} &= \frac{1}{2}\left(\chi_{XX}-\chi_{YY}\pm 2i\chi_{XY}\right) = \frac{1}{2}, \end{aligned} \tag{20}$$

and in the molecular frame

$$\begin{aligned} \chi^{(r)}_{{\rm mol},q} &= \sum_p D^{(r)}_{p,q}\chi^{(r)}_{{\rm lab},p}. \\ &= \sum_p \left(-1\right)^{p-q} D^{(r)*}_{-p,-q}\chi^{(r)}_{{\rm lab},p}. \end{aligned} \tag{21}$$

In addition

$$\begin{aligned} A^{(0)}_{{\rm mol},0} &= -\frac{1}{\sqrt{3}}\left(m_a^2+m_b^2+m_c^2\right) \\ A^{(2)}_{{\rm mol},0} &= \frac{1}{\sqrt{6}}\left(2m_c^2-m_a^2-m_b^2\right) \\ A^{(2)}_{{\rm mol},\pm1} &= \mp\left(m_a m_c \pm m_b m_c\right) \\ A^{(2)}_{{\rm mol},\pm2} &= \frac{1}{2}\left(m_a^2-m_b^2\pm 2i m_a m_b\right). \end{aligned} \tag{22}$$

Finally, the alignment factor is given by

$$\begin{aligned} O\left(t\right) =& A^{(0)}_{{\rm mol},0}D^{(0)*}_{00}\chi^{(0)}_{{\rm lab},0} + A^{(2)}_{{\rm mol},-2}D^{(r)*}_{-p,-2}\chi^{(r)}_{{\rm lab},p} \\ &+ A^{(2)}_{{\rm mol},-1}D^{(r)*}_{-p,-1}\chi^{(r)}_{{\rm lab},p} + A^{(2)}_{{\rm mol},0}D^{(r)*}_{-p,0}\chi^{(r)}_{{\rm lab},p}, \\ &+ A^{(2)}_{{\rm mol},1}D^{(r)*}_{-p,1}\chi^{(r)}_{{\rm lab},p} + A^{(2)}_{{\rm mol},2}D^{(r)*}_{-p,2}\chi^{(r)}_{{\rm lab},p} \end{aligned} \tag{23}$$

where summation over the repeated index $p = -2, \ldots, 2$ is implied. The matrix elements of these expectation values are calculated using Sup. Eq. 15. To include thermal effects, we do ensemble averaging: The initial wave function is set to an eigenstate, $|\Psi(t=0)\rangle = |J\tau M\rangle$, and the expectation values are calculated for this initial state as $P_{J,\tau,M}(t)$ and $O_{J,\tau,M}(t)$. The final expectation value is then the thermally averaged sum

$$P(t) = \sum_{J,\tau,M} P_{J,\tau,M}(t) Z^{-1}\exp\left[-\frac{E_{J,\tau}}{k_B T}\right] \tag{24}$$

$$O(t) = \sum_{J,\tau,M} O_{J,\tau,M}(t) Z^{-1}\exp\left[-\frac{E_{J,\tau}}{k_B T}\right] \tag{25}$$

where $k_B$ is the Boltzmann constant, $T$ the temperature, and $Z = \sum_{J,\tau,M}\exp[-E_{J,\tau}/k_B T]$ is the Canonical partition function. To keep the calculation numerically feasible, only initial states with an angular momentum of $J \le 10$ were included in the ensemble; the expectation values were found to have converged at this value for temperatures of at least $T = 5$ K.

**Supplementary References**

[1] M. J. Frisch, G. W. Trucks, H. B. Schlegel, G. E. Scuseria, M. A. Robb, J. R. Cheeseman, G. Scalmani, V. Barone, G. A. Petersson, H. Nakatsuji, X. Li, M. Caricato, A. V.

Marenich, J. Bloino, B. G. Janesko, R. Gomperts, B. Mennucci, H. P. Hratchian, J. V. Ortiz, A. F. Izmaylov, J. L. Sonnenberg, D. Williams-Young, F. Ding, F. Lipparini, F. Egidi, J. Goings, B. Peng, A. Petrone, T. Henderson, D. Ranasinghe, V. G. Zakrzewski, J. Gao, N. Rega, G. Zheng, W. Liang, M. Hada, M. Ehara, K. Toyota, R. Fukuda, J. Hasegawa, M. Ishida, T. Nakajima, Y. Honda, O. Kitao, H. Nakai, T. Vreven, K. Throssell, J. A. Montgomery, Jr., J. E. Peralta, F. Ogliaro, M. J. Bearpark, J. J. Heyd, E. N. Brothers, K. N. Kudin, V. N. Staroverov, T. A. Keith, R. Kobayashi, J. Normand, K. Raghavachari, A. P. Rendell, J. C. Burant, S. S. Iyengar, J. Tomasi, M. Cossi, J. M. Millam, M. Klene, C. Adamo, R. Cammi, J. W. Ochterski, R. L. Martin, K. Morokuma, O. Farkas, J. B. Foresman, and D. J. Fox. Gaussian 16, Revision A.03, 2016.

[2] Pascal P. Man. Cartesian and spherical tensors in nmr hamiltonians. *Concepts in Magnetic Resonance Part A*, 42(6):197–244, 2013.

[3] A. Yachmenev and S. N. Yurchenko. Detecting chirality in molecules by linearly polarized laser fields. *Phys. Rev. Lett.*, 117:033001, 2016.

[4] Richard Zare. *Angular momentum : understanding spatial aspects in chemistry and physics*. Wiley, New York, 1988.
